# Supplementary material for: Triplet Exciton-driven Topological Mott insulator at Finite Temperature
Source: arXiv:2507.07178 source file (2025-07-18)
Supplement: Supplementary file 1 [file supplement.pdf]

# Triplet Exciton-driven Topological Mott insulator at Finite Temperature: supplemental materials

Peizhi Mai*
*Department of Physics and the Anthony J. Leggett Institute of Condensed Matter Theory, University of Illinois at Urbana-Champaign, Urbana, IL 61801, USA*
(Dated: today)

## CHECKERBOARD QUANTUM-SPIN-HALL HAMILTONIAN

The Hamiltonian for the checkerboard quantum-spin-Hall (QSH) model model is

$$H = \ -t\sum_{\langle \mathbf{ij}\rangle\sigma} e^{\pm i\sigma\psi} c^\dagger_{\mathbf{i}\sigma} c_{\mathbf{j}\sigma} - t'\sum_{\langle\langle \mathbf{ij}\rangle\rangle\sigma} (-1)^{\delta_{\mathbf{i},\mathbf{j}}} c^\dagger_{\mathbf{i}\sigma} c_{\mathbf{j}\sigma} - \mu \sum_{\mathbf{i},\sigma} n_{\mathbf{i}\sigma}, \tag{S1}$$

where the details of the hopping phase and sign convention are given in Fig. S1[1, 2].

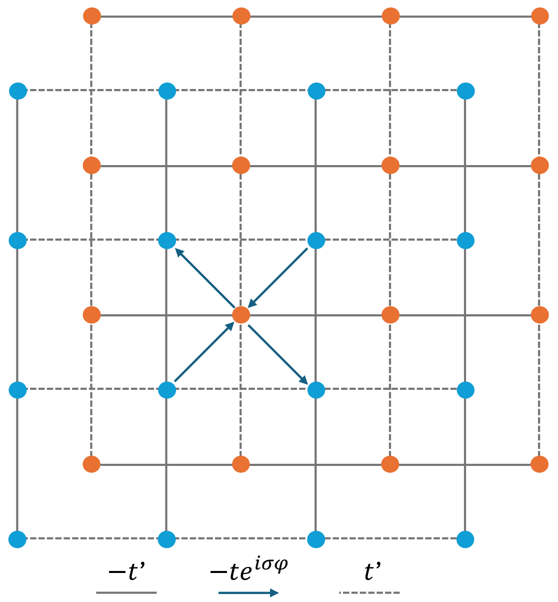


FIG. S1: Hopping parameters and phase convention for the checkerboard QSH model

## CHERN INSULATOR AT $1 < \langle n \rangle < 1.5$ AT HIGH FIELD

In this section, we explore the Chern insulator in the checkerboard QSH model at $1 < \langle n \rangle < 1.5$ induced by high fluxes near $\Phi/\Phi_0 = 0.5$ without interaction, as circled in Fig. S2(a) and shown in the dash line in Fig. S2(b-d). In Fig. S2(b-d), we observe that both spins are present and contribute non-trivial spin-resolved Chern number. The spin-resolved Chern number $C_\sigma$ can be extracted more clearly from the $\chi_\sigma$ shown in Fig. S3. From Fig. S3 (c,d), we learn that for the Chern insulator at $1 < \langle n \rangle < 1.5$ and high flux, $C_\uparrow = 2$ and $C_\downarrow = -1$, leading to a total charge Chern number $C = C_\uparrow + C_\downarrow = 1$.

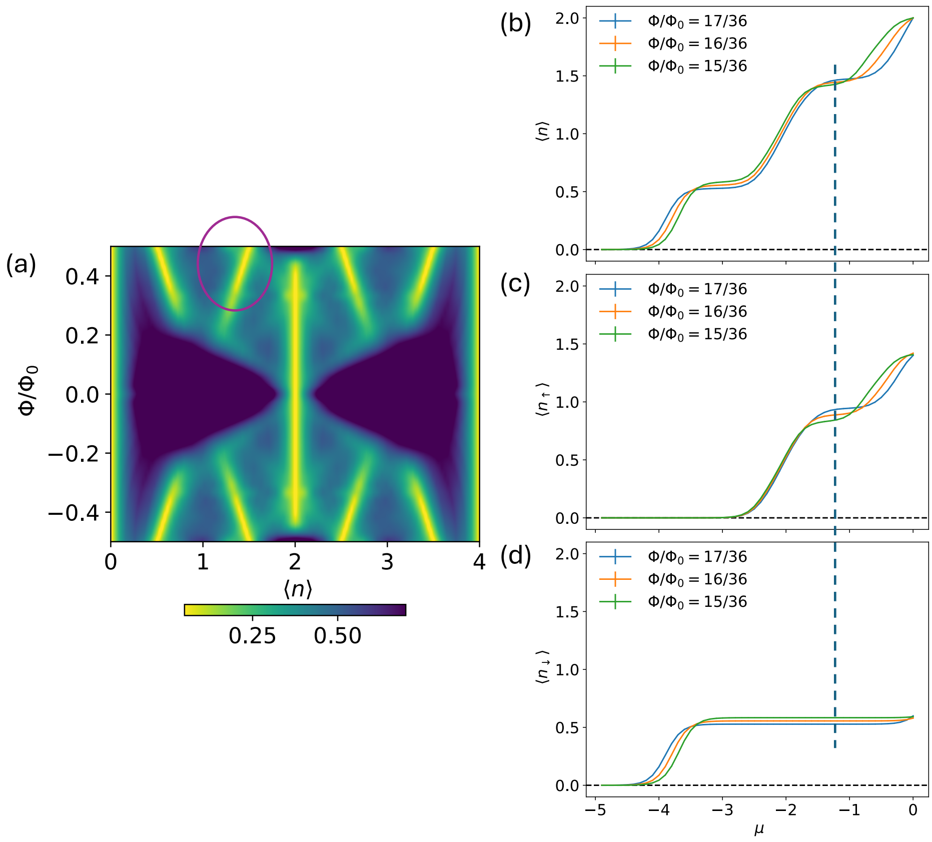


FIG. S2: (a) Compressibility as a function of density $\langle n \rangle$ and magnetic flux $\Phi/\Phi_0$ (b) $\langle n \rangle$ versus chemical potential $\mu$ and (c,d) $\langle n_\sigma \rangle$, both versus chemical potential $\mu$ at high magnetic fields. All panels share the parameters $U = 0$ and $\beta = 8t^{-1}$.

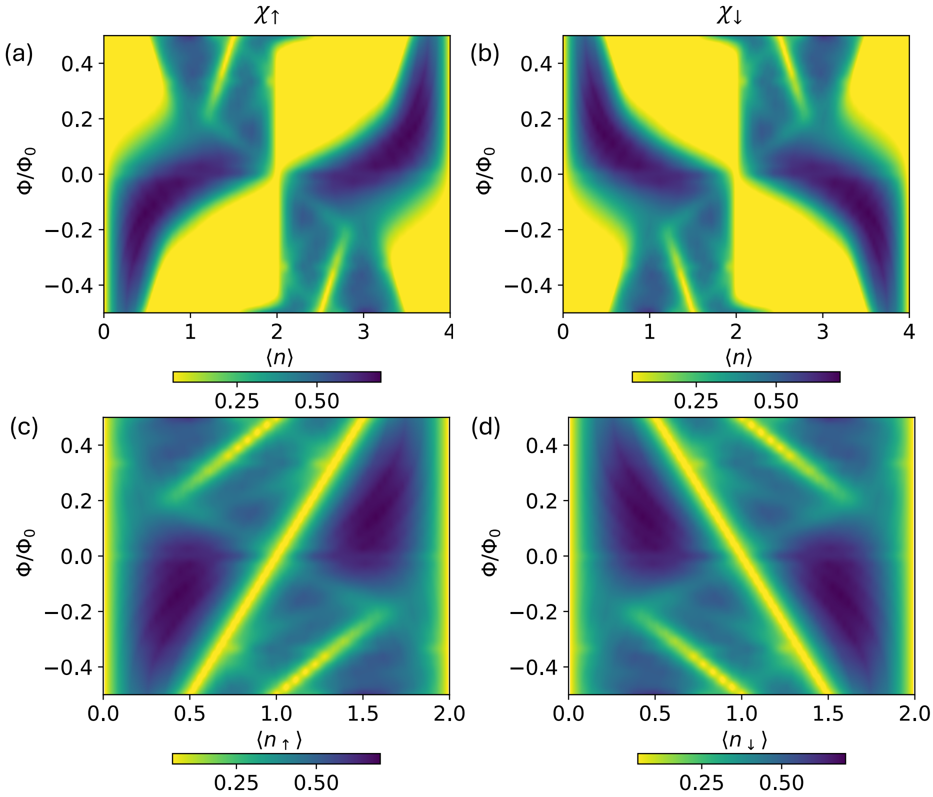


FIG. S3: (a,b) Spin-resolved compressibility $\chi_\sigma$ as a function of density $\langle n\rangle$ and magnetic flux $\Phi/\Phi_0$. (c,d) Spin-resolved compressibility $\chi_\sigma$ as a function of density $\langle n_\sigma\rangle$ and magnetic flux $\Phi/\Phi_0$.

## DETAILS OF DQMC SIMULATIONS

We run our simulations with the open-source DQMC package available at https://github.com/edwnh/dqmc. The inverse temperature $\beta$ is discreted into $L$ slides with step $\Delta\tau = 0.1$. Each Markov chain begins with 10000 warmup sweeps, followed by 200000 measurement sweeps (10 measurements per sweep). To map out the density dependence, we vary the chemical potential from $-5$ to $5$ in steps of $0.05 \sim 0.1$. The severity of the sign problem (see Fig. S4) dictates how many independent Markov chains we average: between 10 and 1000, with more chains used when the average sign is small.

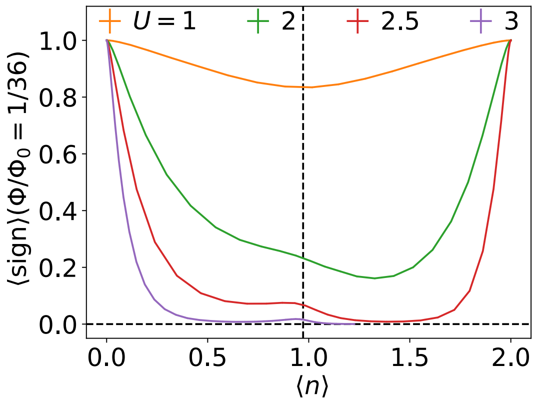


FIG. S4: Average sign from DMQC simulation on the checkerboard QSH-Hubbard model under a minimal magnetic flux $\Phi/\Phi_0 = 1/36$ in a $6 \times 6 \times 2$ cluster at $\beta = 8t^{-1}$ with varying $U$.

## FERROMAGNETIC TRANSITION

We fix $U = 2.5, \beta = 8$ and plot the Spin susceptibility $\chi_s$ as a function of density $\langle n \rangle$ and magnetic flux $\Phi/\Phi_0$ in Fig. S5(a). A pronounced peak appears near zero field and quarter filling $\langle n \rangle = 1$, indicating strong ferromagnetic (FM) fluctuations, though not long-range FM order. To probe the onset of magnetism, we calculate the temperature evolution of $1/\chi_s$ with $U = 3$ in Fig. S5(b). The rapid decrease of $1/\chi_s$ with decreasing temperature $T$ suggests a divergence of $\chi_s$ at a finite Curie temperature $T_c \approx 0.65$ or $\beta_c \approx 15$, as shown by the extrapolation dashed curve. This trend is consistent with the DQMC results in the Kane–Mele–Hubbard model[3].

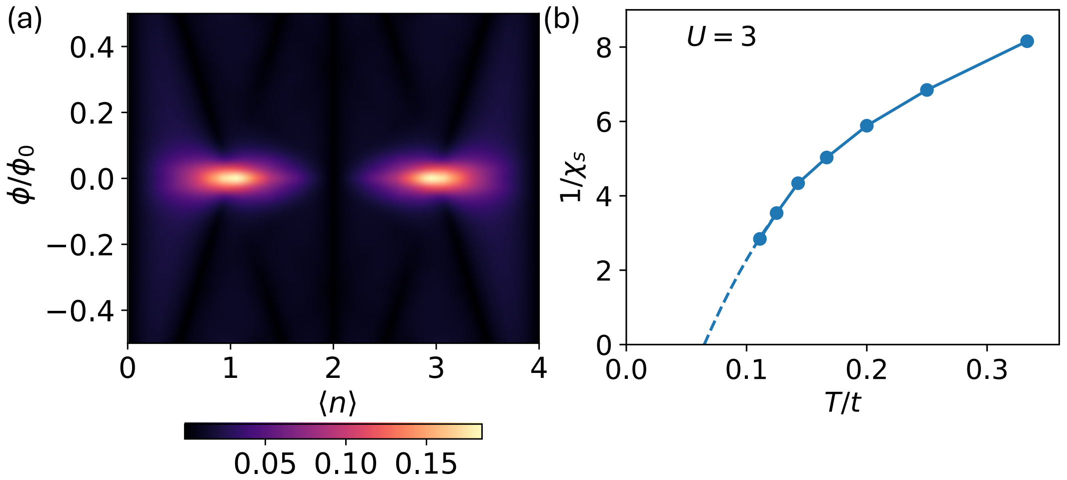


FIG. S5: (a) Spin susceptibility $\chi_s$ as a function of density $\langle n \rangle$ and magnetic flux $\Phi/\Phi_0$ at $U = 2.5t, \beta = 8t^{-1}$ (b) $1/\chi_s$ versus temperature at $U = 3$ and zero field.

* Electronic address: peizhimai@gmail.com

[1] T. Neupert, L. Santos, C. Chamon, and C. Mudry, Phys. Rev. Lett. **106**, 236804 (2011), URL `https://link.aps.org/doi/10.1103/PhysRevLett.106.236804`.
[2] K. Sun, Z. Gu, H. Katsura, and S. Das Sarma, Phys. Rev. Lett. **106**, 236803 (2011), URL `https://link.aps.org/doi/10.1103/PhysRevLett.106.236803`.
[3] P. Mai, J. Zhao, B. E. Feldman, and P. W. Phillips, Nature Communications **14**, 5999 (2023).
